# Supplementary material for: Surface plasmon polariton assisted optical pulling force
Source: arXiv:1601.01863 ancillary file (2016-01-08)
Supplement: Supplementary file 1 [file Supplementary.pdf]

Supporting Information

# Plasmonic negative forces

*Mihail I. Petrov[1], Sergey V. Sukhov[2], Andrey A. Bogdanov[1,3,4], Alexander S. Shalin[1,5,6,*], Aristide Dogariu[2,*]*

[1]The International Research Centre for Nanophotonics and Metamaterials, ITMO University, St Petersburg, Russia

[2]CREOL, The College of Optics and Photonics, University of Central Florida, 4000 Central Florida Blvd., 32816 Orlando, Florida, USA

[3]Ioffe Institute, St Petersburg, Russia

[4]Peter the Great St. Petersburg Polytechnic University, St Petersburg, Russia

[5]Kotel'nikov Institute of Radio Engineering and Electronics of Russian Academy of Sciences (Ulyanovsk branch), Ulyanovsk 432011, Russia

[6]Ulyanovsk State University, Ulyanovsk, Russia

**Table of Content**

- Dyadic Green's function of a particle placed above a plasmonic interface
- Expression for the force acting on a particle placed above a plasmonic interface
- Calculation of the integral entering the expression of derivative of the Green's function for specific cases
- Polarizability of a dipole near the interface
- Mapping the angular and spectral dependence of the $F_z$ component
- Description of movie

## A. Dyadic Green's function

The diagonal components of the reflected Green's function calculated at the origin $\hat{G}^R(\mathbf{r}_0,\mathbf{r}_0)$ can be expressed as follows[1]:

$$k_z = \sqrt{k^2 - k_\parallel^2}, \quad k_{zs} = \sqrt{\varepsilon_{21}k^2 - k_\parallel^2}, \varepsilon_{21} = \varepsilon_s / \varepsilon_m \qquad r_s = \frac{k_z - k_{zs}}{k_z + k_{zs}}, \quad r_p = \frac{\varepsilon_{21}k_z - k_{zs}}{\varepsilon_{21}k_z + k_{zs}} \tag{1}$$

$$\hat{G}_{xx}^R(\mathbf{r}_0,\mathbf{r}_0) = \frac{ik}{8\pi}\int_0^\infty \frac{k_\parallel}{k_z}\left(r_s(k_\parallel) - \frac{k_z^2}{k^2} r_p(k_\parallel)\right)\exp(2ik_z z_0)dk_\parallel, \tag{2}$$

$$\hat{G}_{zz}^R(\mathbf{r}_0,\mathbf{r}_0) = \frac{i}{4\pi k}\int_0^\infty \frac{k_\parallel^3}{k_z} r_p(k_\parallel)\exp(2ik_z z_0)dk_\parallel, \tag{3}$$

where $k$ is the wavenumber, $k_\parallel$ and $k_z$ are the wavevector components lateral and normal to the interface, $z_0$ is the distance from the dipole to the interface between the media, the permittivity of upper space is taken equal to 1 similarly to the main body text.

## B. Forces created by the rescattered field

In this section we derive the expressions for longitudinal $F_x^D$ and normal to the interface $F_z^D$ forces created by a dipole radiation scattered back from the substrate. The expression for the optical force in the dipole approximation is as follows:

$$F_x^D = \frac{1}{2}\mathrm{Re}\left(\mathbf{p}^* \frac{\partial \mathbf{E}^D}{\partial x}\right), \quad F_z^D = \frac{1}{2}\mathrm{Re}\left(\mathbf{p}^* \frac{\partial \mathbf{E}^D}{\partial z}\right) \tag{4}$$

The dipole field $E^D$ is defined by the components of the dipole moment and Green's function $\hat{G}^R$:

$$E_x^D(\mathbf{r}) = \frac{k^2}{\varepsilon_0}\left(\hat{G}_{xx}^R(\mathbf{r},\mathbf{r}_0)p_x + \hat{G}_{xz}^R(\mathbf{r},\mathbf{r}_0)p_z\right), \tag{5}$$

$$E_z^D(\mathbf{r}) = \frac{k^2}{\varepsilon_0}\left(\hat{G}_{zz}^R(\mathbf{r},\mathbf{r}_0)p_z + \hat{G}_{zx}^R(\mathbf{r},\mathbf{r}_0)p_x\right). \tag{6}$$

To calculate forces $F_x^D$, $F_z^D$, one need to compute the *x*- and *z*-derivatives of the Green's function $\partial_x \hat{G}_{xx,zz,xz}^R$ at the location of the dipole $\mathbf{r} = \mathbf{r}_0$. The derivative of diagonal components of tensor vanishes at the location of a dipole $\partial_x \hat{G}_{xx,zz}^R(\mathbf{r}_0,\mathbf{r}_0) = 0$, thus the field derivative computed at the location of the dipole has the form:

$$\partial_x E_x^D(\mathbf{r}_0) = \frac{k^2}{\varepsilon_0}\partial_x \hat{G}_{xz}^R(\mathbf{r}_0,\mathbf{r}_0)p_z \qquad \partial_x E_z^D(\mathbf{r}_0) = \frac{k^2}{\varepsilon_0}\partial_x \hat{G}_{zx}^R(\mathbf{r}_0,\mathbf{r}_0)p_x \tag{7}$$

Taking into account that $\hat{G}^R_{xz} = -\hat{G}^R_{zx}$, one can get the following expression for the longitudinal force

$$F_x^D = -\frac{k^2}{\varepsilon_0}\mathrm{Im}(p_x^* p_z)\mathrm{Im}\left(\partial_x \hat{G}^R_{xz}\right). \tag{8}$$

Far from configurational resonances[2,3], $p_x \approx \alpha_0 E_x^0$, $p_z \approx \alpha_0 E_z^0$, and $\mathrm{Im}(p_x^* p_z)$ can be written as

$$\mathrm{Im}(p_x^* p_z) = |\alpha_0|^2 |E^0|^2 \sin 2\theta \,\mathrm{Im}\left[r_p \exp\left(2ik_1 z_0 \cos\theta\right)\right]. \tag{9}$$

Assuming $r_p = \exp(2i\phi)$ for metallic substrates, after some simple algebra one can find that

$$\mathrm{Im}(p_x^* p_z) = |\alpha_0|^2 |E^0|^2 \sin 2\theta \sin\left[2(k_{z1} z_0 + \phi)\right]. \tag{10}$$

From this expression one can see that $F_x^D$ is dependent on the dipole position $z_0$. That means that under some conditions that still to be specified the sign of $F_x^D$ can be negative!

Computing $z$-component of the field, one should take into account that $\partial_z \hat{G}_{xz}(\mathbf{r}_0, \mathbf{r}_0) = 0$. Thus, we obtain

$$F_z^D = \frac{k^2}{2\varepsilon_0}\left(|p_x|^2 \,\mathrm{Re}\,\partial_z \hat{G}^R_{xx} + |p_z|^2 \,\mathrm{Re}\,\partial_z \hat{G}^R_{zz}\right). \tag{11}$$

Here we list the required expressions for Green's function components in the notations used in section S1:

$$\partial_x \hat{G}^R_{xz}(\mathbf{r}_0, \mathbf{r}_0) = \frac{1}{8\pi k^2}\int_0^\infty k_\parallel^{\,3} r_p(k_\parallel) \exp(2ik_z z_0) dk_\parallel, \tag{12}$$

$$\partial_z \hat{G}^R_{xx}(\mathbf{r}_0, \mathbf{r}_0) = \frac{1}{8\pi k^2}\int_0^\infty k_\parallel (k^2 r_s(k_\parallel) - k_z^2 r_p(k_\parallel)) \exp(2ik_z z_0) dk_\parallel, \tag{13}$$

$$\partial_z \hat{G}^R_{zz}(\mathbf{r}_0, \mathbf{r}_0) = \frac{1}{4\pi k^2}\int_0^\infty k_\mathrm{P}^3 r_p(k_\mathrm{P}) \exp(2ik_z z_0) dk_\mathrm{P}. \tag{14}$$

## C. Calculation of the integral entering the expression of derivative of the Green's function for specific cases

To gain some insights about the magnitude of the force $F_x^D$ in Eq. (8), one should evaluate the integral entering the expression for $\mathrm{Im}\,\partial_x \hat{G}^R_{xz}$ [Eq. (12)]. Here we estimate it for the case of a substrate with negative permittivity $\varepsilon_s < 0$ without losses. Although this is an idealization, it will allow us to estimate the contribution of the surface plasmon polariton (SPP) to the force $F_x^D$. The integral in Eq. (12) can be divided into two parts:

$$\partial_x \hat{G}^R_{xz}(\mathbf{r}_0,\mathbf{r}_0) = \frac{1}{8\pi k^2}\int_0^k k_\parallel{}^3 r_p(k_\parallel)\exp(2ik_z z_0)dk_\parallel + \frac{1}{8\pi k^2}\int_k^\infty k_\parallel{}^3 r_p(k_\parallel)\exp(2ik_z z_0)dk_\parallel$$
$$= \partial_x \hat{G}^{R0}_{xz}(\mathbf{r}_0,\mathbf{r}_0) + \partial_x \hat{G}^{R-SPP}_{xz}(\mathbf{r}_0,\mathbf{r}_0), \quad (15)$$

The integration range $0 < k_\text{P} < k$ in $\partial_x \hat{G}^{R0}_{xz}$ corresponds to the propagating waves in the upper space. To analyze the interaction of the nanoparticle with the SPP and to isolate the SPP contribution into the total optical force we also introduce SPP Green's function $\hat{G}^{R-SPP}_{xz}$ by integrating the $k_\text{P}$-space over the evanescent modes $k_\text{P} > k$ .

Propagating surface plasmon exists only for $\varepsilon_s < -\varepsilon_m$. Reflection coefficient $r_p(k_\text{P})$ has a pole $k_{SPP} = k\sqrt{\varepsilon_m \varepsilon_s / (\varepsilon_s + \varepsilon_m)} > k$ corresponding to the excitation of surface plasmon polariton located on a real axis in the region of evanescent modes.

Let us consider the integral of the following form

$$\int_k^\infty h(k_\parallel) r_p(k_\parallel)\exp(2ik_{z1}z_0)dk_\parallel = \int_k^\infty h(k_\parallel)\frac{g_p(k_\parallel)}{k_\parallel - k_{SPP}}\exp(-2\sqrt{k_\parallel^2 - k^2}z_0)dk_\parallel, \quad (16)$$

where $h(k_\parallel)$ is a function without singularities and $g_p(k_\parallel)$ is the regular part of the reflection coefficient. As the pole is located on the integration axis, one should regularize the divergence and shift the pole away from the axis using the expression:

$$\frac{1}{x - i0} = v.p.\frac{1}{x} + \pi i \delta(x). \quad (17)$$

Then the integral in Eq. (16) becomes

$$(16) = v.p.\int_k^\infty h(k_\parallel)\frac{g_p(k_\parallel)}{k_\parallel - k_{SPP}}\exp(-2\sqrt{k_\parallel^2 - k^2}z_0)dk_\parallel + \pi i\ h(k_{SPP})g_p(k_{SPP})\exp(-2\sqrt{k_{SPP}^2 - k^2}z_0). \quad (18)$$

One can see that the second term contains imaginary unit that ensures nonzero value of expression $\partial_x \hat{G}^{R-SPP}_{xz}$ in $k_\parallel \in [k,\infty)$ integration range. In particular, the imaginary part of Green's function can be estimated as

$$h(k_{SPP}) = k_{SPP}^3 \quad , \quad g_p(k_{SPP}) = \frac{2|\varepsilon_{21}|^{3/2} k_{SPP}}{\sqrt{|\varepsilon_{21}| - 1}\left(|\varepsilon_{21}|^2 - 1\right)},$$
$$\operatorname{Im}\partial_x \hat{G}^{R-SPP}_{xz}(\mathbf{r}_0,\mathbf{r}_0) = \frac{1}{8k^2} h(k_{SPP}) g_p(k_{SPP}) \exp\left(-2\sqrt{k_{SPP}^2 - k^2}z_0\right) \approx \frac{k_{SPP}^2}{8}\frac{k_{SPP}^5}{k^5}\exp\left(-2\sqrt{k_{SPP}^2 - k^2}z_0\right) \quad (19)$$

Next we have computed the imaginary part of the Green's function for the case of metal within the Drude model $\varepsilon_s = \varepsilon_\infty - \omega_p^2 / \omega(\omega + i\gamma)$ for following parameters: $\varepsilon_\infty = 4$, $\omega_p = 9$ eV, which corresponds to Drude parameters of silver. The imaginary part of the Green's function calculated via numerical integration of the integral (15) (solid line) and with formula (19) (dashed line) is shown in Figure S1 for the case of

lossless metal $\gamma = 0$ and for low losses $\gamma = 10^{-2}\omega_p$. One can see that the imaginary part of the Green's function derivative can be described by the expression (19) even accounting for losses. The imaginary part of $\partial_x \hat{G}_{xz}^{R0}(\mathbf{r}_0, \mathbf{r}_0)$ is not show in Figure S1 as it is as small as $10^{-3}$.

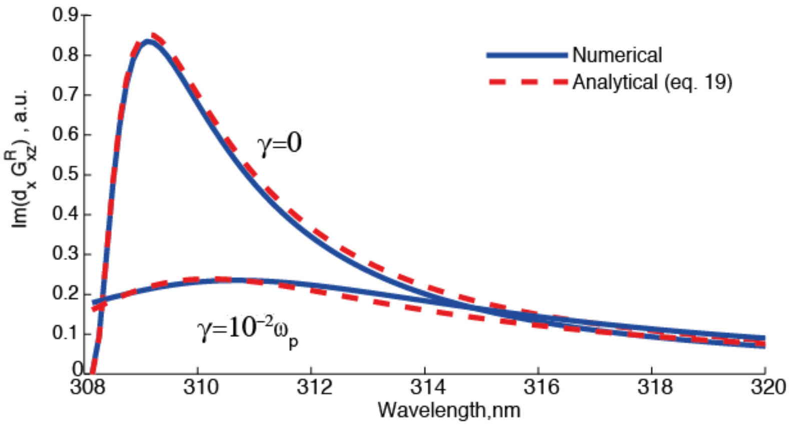


Figure S1. Contribution of the evanescent (SPP) modes into imaginary part of the Green's function derivative for Drude metal with the parameters $\varepsilon_m = 1,\ \varepsilon_\infty = 4,\ \omega_p = 9eV,\ \gamma = 0;\ 10^{-2}\omega_p$. The wavelength of SPP at the interface with air $\lambda_{SPP} = \omega_p / \sqrt{\varepsilon_m + \varepsilon_\infty} = 308$ nm.

Finally, far from configurational resonance we can use expression (10) and obtain the approximate formula for the lateral force related to SPP generation:

$$F_x^D = -\frac{k_{SPP}^4 k_{SPP}^3}{8\varepsilon_0 \ k^3} |\alpha_0|^2 |E^0|^2 \sin 2\theta \sin\left[2(k_z z_0 + \phi)\right] \exp\left(-2\sqrt{k_{SPP}^2 - k^2} z_0\right). \qquad (20)$$

One should note that according to (20) at the SPP resonance, i.e. $\varepsilon_s \to -\varepsilon_m,\ k_{SPP} \to \infty$, the force becomes equal to zero because of the exponent factor. The spectral maximum of the negative force is shifted into the long wavelength range where the maximum of expression (20) is observed. Moreover, the lateral force decays very fast away from it as exponential factor becomes very small. Thus, the maximum of the lateral force for finite size particles is red shifted.

## D. Polarizability of a dipole near the interface

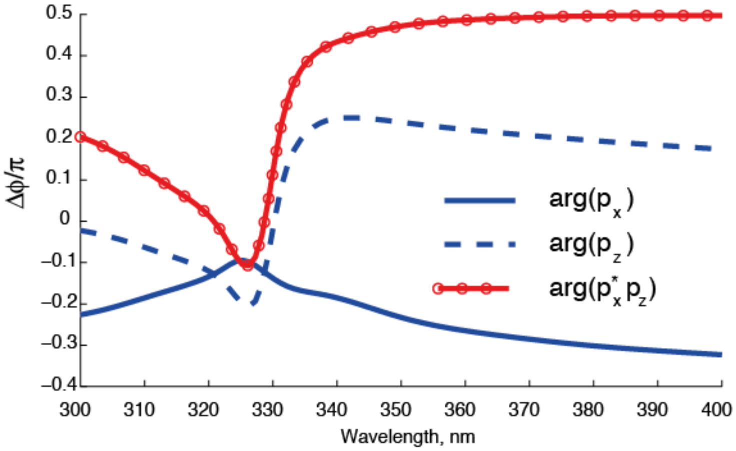


Figure S2. The spectral dependence of the phases of $p_x$ and $p_z$ dipole components for dielectric particle with radius 15 nm and dielectric permittivity $\varepsilon = 3$ placed in air above a silver surface at $z_0 = 27$ nm, and for the angle of incidence $\theta = 35°$.

The $\pi / 2$ phase shift between $p_x$ and $p_z$ (red line with circles in Figure S2) results in rotating dipole picture, which one can clearly see from the video-file attached to the Supplementary Materials. The rotating dipole moment of nanoparticle is responsible for directional excitation of SPP.

## E. Mapping the angular and spectral dependence of the $F_z$ component

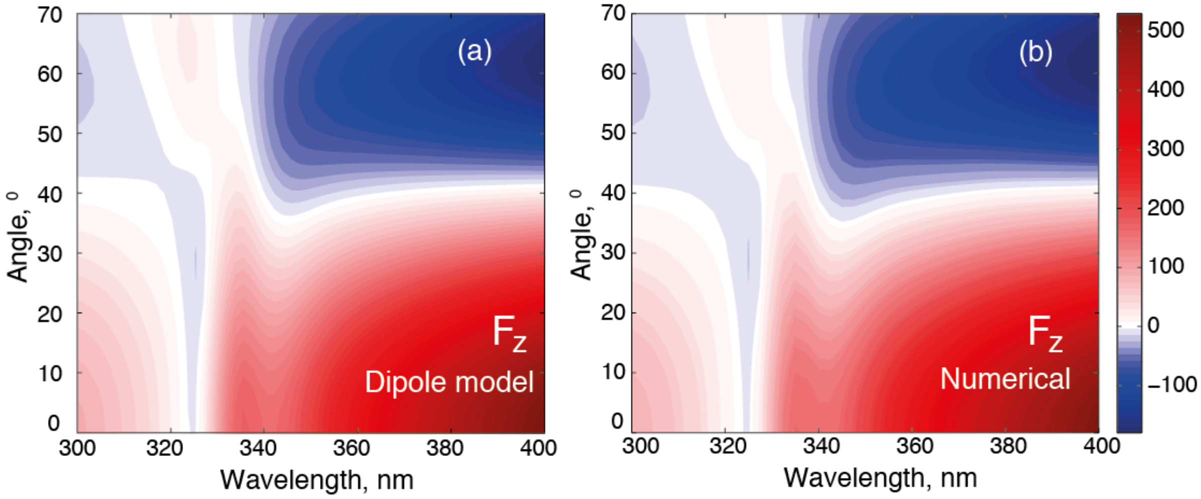


Figure S3. The components of the optical force normal to the interface computed for different wavelengths and incidence angles within the analytical dipole model (a) and numerically (b). The parameters of calculation are the same as in Figure 2. The force $F_z$ is given in units of $F_0$.

## F. Description of movie

The provided Supplementary movie shows time dependence of magnetic filed component $H_z^D$ (z-direction is perpendicular to the figure plane) of the scattered field induced by the TM-polarized wave incident at angle $\theta = 35^\circ$ with wavelength $\lambda = 400$ nm. Scattered field includes dipole radiation and SPP field. Dielectric particle placed in air above the silver substrate at $z_0 = 27$ has radius $R = 15$ nm and dielectric permittivity $\varepsilon = 3$. Dielectric permittivity of silver is taken from Ref. 4. The simulation was done using Comsol Multyphysics.

# References

[1] Novotny, L.; Hecht, B. *Principles of Nano-Optics*, Cambridge University, 2006.
[2] Keller, O.; Xiao, M.; Bozhevolnyi, S. Configurational resonances in optical near-field microscopy: a rigorous point-dipole approach. *Surf. Sci.* **1993,** 280, 217–230.
[3] Moiseev, S. G. Configurational resonances phenomena in optical scattering spectroscopy of nano-objects. *Proc. of SPIE*, **2002**, 4748, 419-428.
[4] Johnson, P.B.; Christy, R.W. Optical Constants of the Noble Metals. *Phys. Rev. B* **1972**, 6, 4370-4379.
